# Supplementary material for: Localization and Mapping using Instance-specific Mesh Models
Source: arXiv:2103.04493 source file (2021-03-08)
Supplement: Supplementary file 1 [file Appendix.tex]

\section{}
\label{app:a}
\begin{proof}[Proof of Lemma~\ref{lem:1}]
We proceed by induction.
\end{proof}

\section{}
\label{app:b}
\begin{proof}[Proof of Thm.~\ref{thm:1}]
We proceed by contradiction.
\end{proof}
